# Supplementary material for: The Statistical Model for Ticker, an Adaptive Single-Switch Text-Entry Method for Visually Impaired Users
Source: arXiv:1804.07777 source file (2018-04-20)
Supplement: Supplementary file 1 [file appendix.pdf]

# Supplemental Material for Ticker: An Adaptive Single-Switch Text-Entry Method for Visually Impaired Users

Emli-Mari Nel  
University of Cambridge  
en256@cam.ac.uk

Per Ola Kristensson  
University of Cambridge  
pok21@cam.ac.uk

David J. C. MacKay  
University of Cambridge  
djcm1@cam.ac.uk

**Index Terms**—single-switch systems, accessibility, augmentative and alternative communication, Bayesian inference.

## I. THE AUDIO SEQUENCE FOR $R = 2$

We focus on  $R = 2$ , where a large variety of noise can be accommodated. This setting is intended for situations where the user is conscious and has the capability to memorise the audio sequence. A typical user would be *compos mentis*, and use, for example, a blink detector to click within a few seconds of when they intend to.

Due to the serial nature the interface for this application, it is difficult to come up with a technique that adapts to the interface dynamically (so that more probable words/letters are easier to select) without increasing the cognitive load too much. We therefore assume the audio sequence to be fixed so that the user can pre-empt when a certain letter will be pronounced. We assume the letters occur in alphabetical order for  $r = 1$ , so that the user only has to memorise the sequence for  $r = 2$ . For example, in Figure 2 the letter sequence *abcde* is associated with  $r = 1$ . The user has to then memorise *deabc* for  $r = 2$ .

If the user's click-time precision is noisy, it can be difficult to make an estimate of the intended letter after just one click. If the letters that were close to the intended letter at  $r = 1$  occur far away from it at  $r = 2$ , disambiguation can become remarkably easier. Hence, to compute the audio sequence for  $r = 2$ , the distances between letters that were close to each other for  $r = 1$  should be large for  $r = 2$ . Since all sound files are assumed to have the same length, one can integerise this computation, considering the number of letters between certain letter pairs. For example, in Figure 2, letters  $r$  and  $x$  are adjacent when  $r = 1$ , and are separated by five letters when  $r = 2$ .

The total number of letters  $AR$  is not always divisible by the number of channels. This can cause the characters to sound arrhythmic at the beginning and end of the within-channel sequence, making it more difficult to tune in on a voice. To account for this, some sound files at the beginning/end of a sequence were made slightly longer. To further assist the user to control his/her timing, two “tick” sounds were added at the beginning of the audio sequence to set the pace of the rhythm. The adjusted sound-file lengths and the addition of the “tick” sounds were not

part of the interface during the initial user trials. These adjustments were made after feedback from the users, and resulted in a significant improvement.

The computation of the audio sequence is performed in two steps. Firstly, the  $K$  nearest neighbours of each letter  $\ell$  are stored for  $r = 1$ . Secondly, the sequence for  $r = 2$  is chosen such that all of the stored neighbours from the first step are at least  $K$  letters away from  $\ell$ . This process is repeated to maximise  $K$ . It was found that for 1–5 channels, the maximal  $K$  are (4, 4, 4, 3, 3), respectively.

There can be several sequences with the same  $K$ . Some of the sequences were further eliminated by restricting successive sound pairs, as some sounds can become indistinguishable when they overlap. Sequences containing any of the pairs  $\{a, h\}$ ,  $\{q, k\}$ ,  $\{m, n\}$ ,  $\{b, d\}$  and  $\{a, i\}$  were removed.

Dasher and Nomon both rely on the parallel display capabilities on a computer screen. Due to the serial nature of an audio interface for single-switch users, it is difficult to come up with a technique that adapts the interface dynamically (so that more probable words/letters are easier to select) without increasing the cognitive load too much. If  $R \leq 2$ , it should be assumed the user can click fairly precisely (with a large degree of consistency). If the user can cope with multiple audio channels, the fastest speed can be obtained by fixing the audio sequence. The audio sequence is then typically easy to memorise, which may result in a significant boost in text-entry rate.

This section focusses on the computation of the audio sequence for 1–5 audio channels and  $R = 2$ . Note that  $R = 2$  is analogous to the average of 2 cpc that were necessary during our informal Nomon user trials discussed in Section ?? (controlled by facial gestures). Selecting  $R$  depends on the noise at hand. A large variety of noise can be accommodated for  $R = 2$ , and is intended for situations where the user is conscious and has the capability to memorise the audio sequence. A typical user would be *compos mentis*, and use, e.g., a blink detector to say “yes\_” within a few seconds when he/she intends to.

With  $R = 1$  the most intuitive audio sequence would be the conventional alphabetical order. This setting is only viable if there is virtually no noise in the system, and is not considered practical.

When  $R > 2$  it can become strenuous to memorise the audio sequence. Such cases will typically correspond to a very noisy situation, such as when the user is unconscious and the switch events are slow and difficult to detect, or when users are severely disabled. In such cases the resulting click times typically have large standard deviations. It may then be more viable to reduce the speed slightly and make use of an adaptive audio sequence. For initial testing, the first repetition of all letters can perhaps be in alphabetical order, after which one can use the Uniform distribution to sample the remaining part of the audio sequence. One can then proceed to use Equation ?? as an improvement to compute a more suitable pseudo-random audio sequence (similar to Nomon).

For  $R = 2$ , the audio sequence is determined by firstly assuming the letters for  $r = 1$  are in alphabetical order, so that the user only has to memorise the sequence for  $r = 2$ . For example, in Figure 2 *abcde* is associated with  $r = 1$ , which makes it easy to memorise *deabc* when  $r = 2$ .

If the user's click-time precision is noisy, it can be difficult to make an estimate of the intentional letter after just one click. If the letters that were close to the intentional letter when  $r = 1$  occur far away from it when  $r = 2$ , disambiguation can become remarkably easier. Hence, to compute the audio sequence for  $r = 2$ , the distances between letters that were close to each other when  $r = 1$  are maximised when  $r = 2$ . Since all sound files are assumed to have the same length, one can integerise this computation, considering the number of letters between certain letter pairs. For example, in Figure 2, "r" and "x" are adjacent when  $r = 1$ , and are separated by four letters when  $r = 2$ .

The computation of the audio sequence is performed in two steps. Firstly, the letters  $\ell'_\ell$ , corresponding to the  $K$  nearest neighbours of  $\ell$  are stored for  $r = 1$ :

$$\ell'_\ell = \{\ell' : a_{\ell_1} - a_{\ell'_1} \leq K\}, \quad (1)$$

where  $a_{\ell_1}$  indicates that  $\ell$  is the  $a$ 'th letter in the audio sequence when  $r = 1$ . The sequence for  $r = 2$  is then optimised so that, for any  $\ell_1$ , any one of its  $K$  nearest neighbours (i.e., any letter in  $\ell'_\ell$ ) is at least  $K$  letters from  $\ell_2$ , where  $K$  is maximised. It was found that for 1-5 channels,  $K = \{4, 4, 4, 3, 3\}$ , respectively.

There can be several sequences with the same  $K$ . Some of the sequences were further eliminated by restricting successive sound pairs, as some sounds can become indistinguishable when they overlap. Sequences containing any of the pairs  $\{a, h\}$ ,  $\{q, k\}$ ,  $\{m, n\}$ ,  $\{b, d\}$  and  $\{a, i\}$  were removed.

The number of letters  $AR$  is not always divisible by the number of channels. This can cause the characters to sound asynchronous at the beginning and end of the within-channel sequence, making it more difficult to tune in on a voice. To account for this some sound files at the beginning/end of a sequence were made slightly longer. To further assist the user to control his/her timing, two "tick" sounds were added at the beginning of the audio sequence. Adjusting the sound-file length and adding the "tick" sounds were not added in the initial user trials, but

due to feedback received from them, and resulted in a great improvement.

Figure 1(a) depicts the final audio sequences in 2D, where the beginning of the sound file of each letter is plotted for  $r = 1$  (first dimension) and  $r = 2$  (second dimension). With this visualisation one can get a clear impression of the nearest neighbours of each letter. The "tick" sounds were added at the beginning of each sequence, and the length of all sound files are 1 second, except for a small number of cases. Letters that are close to one another in 2D will be more difficult to distinguish from one another if the user does not click with high precision. Note however, that the shown audio-sequence times do not correspond to typical user times. An expert user would, for example, operate at a speed of almost 8 times faster in 5 channels, where it will take 5 seconds to repeat the alphabet twice instead of the shown 40 seconds.

It should be noted that our optimisation of the audio sequence corresponds to maximisation of Equation ??, and that some simplifying assumptions were made to construct our approach. These assumptions were made to reduce computational cost, and increase generality of use. By clarity of hindsight, some major improvements can be made by alleviating some of these assumptions.

Firstly, we have assumed that  $P(X)$  is the Uniform distribution, thereby ignoring our dictionary. When one does not ignore the dictionary, it can naturally lead to sequences where the separation between letter pairs that are frequently close to each other are increased. It may then become much easier to select frequently occurring words, thereby increasing the overall text-entry speed. Note from Figure 1(a) that "o" and "e" are close to each other when considering all sound pairs in the 5-channel configuration. In English, these two vowels frequently occur next to each other. By default, pairs like "o" and "e" would therefore limit the performance of the system by definition, if the user writes in English.

Ignoring a dictionary with more than a hundred thousand words, when optimising Equation ??, reduces the computational considerably, so that one only has to consider letter codewords (such as shown in Figure 1(b)) for all the possible input letters (not all possible words). Initially it was thought the simplification is perhaps sub-optimal if the user's preferred language is known, but that it does accommodate a simplified setting, where any letter in the alphabet could be mapped to acronyms for actions (of equal probability), e.g., "a" could be used to "turn on the TV". In hindsight it would have been better to include the dictionary, since the capability to communicate freely and to a full extent with a higher accuracy, far outweighs the simplicity to select a small number of actions.

Some simplifying assumptions of less significance during the optimisation of the audio sequence were: the audio files of all letters were assumed to have the same length, making the denominator in Equation ?? irrelevant. False positive and false negative switch noise were ignored (assuming the user clicks exactly  $R$  times for each letter). A rudimentary click-time model was also assumed.

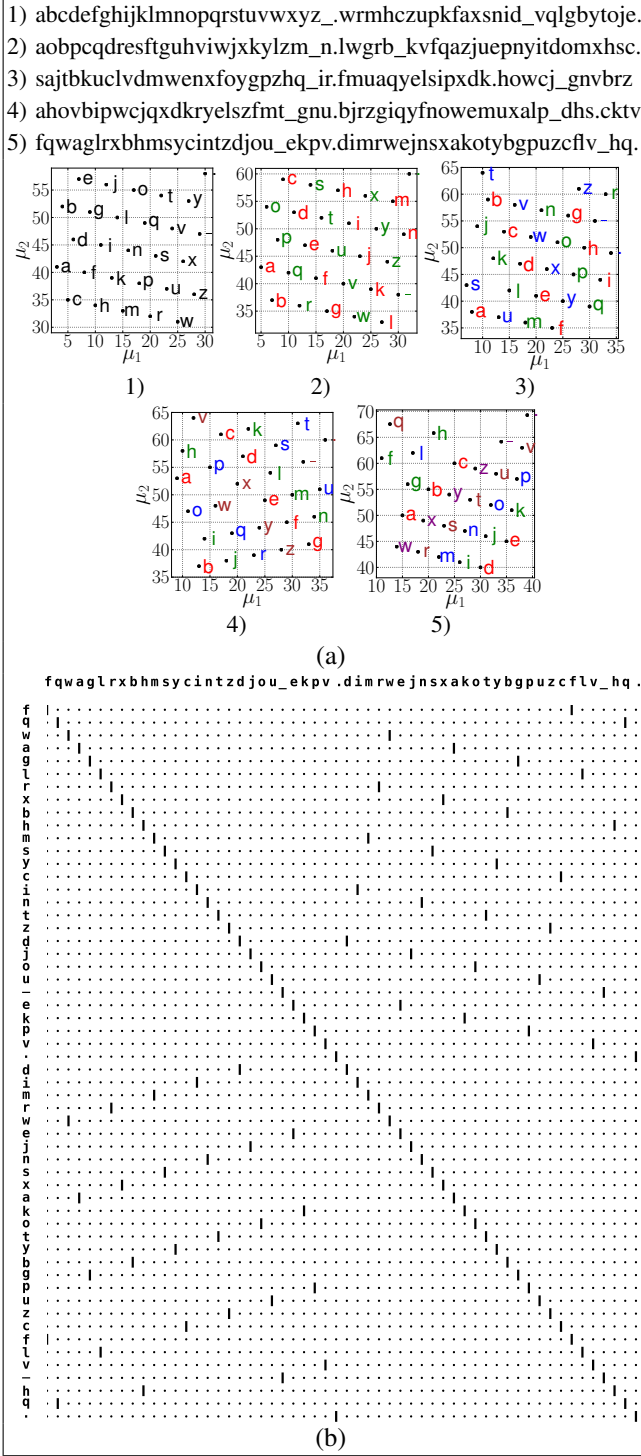

Fig. 1. (a) The final audio sequences for 1-5 channels and their corresponding 2D plots. Letters from the same channel are represented by the same colour. The beginning of each sound file for  $r = 1$  ( $\mu_1$ ) is plotted against the beginning of each sound file for  $r = 2$  ( $\mu_2$ ), where  $\mu_1$  and  $\mu_2$  are measured in seconds. (b) The codewords associated with all letters in the alphabet for 5 channels (as part of computing the audio sequence). The y-axis indicates the desired letter, whereas the x-axis indicates which letter to select ("1") or not to select ("0").

Note that the above simplifications were not applied when doing inference in Ticker, but only during the optimisation of the audio sequence. During inference a much more comprehensive noise model is used (as described

in Section ??) to allow for more interesting and smooth click-time models, and which can also adapt to the user. The letter priors are also not ignored during inference.

Figure 2(f) illustrates that each word in the dictionary has a unique pseudo-random binary code. Each letter is associated with a dot or line: The dot represents a zero, and is associated with the letters that the user should not select while the audio sequence is presented. The lines represent the timings of the desired letters (indicating when the user has to click). The system is optimal if the distances between confusing, frequently occurring letters are maximised in binary symbol space. For example, if "ace\_" and "act\_" shown in Figure 2(d) both have similar (large) prior probability mass, the ones associated with  $e$  and  $t$  should ideally be as far from each other as possible.

## II. DERIVATION OF THE CLICK-TIMING DISTRIBUTION FOR THE SIMPLE MODEL

From the generative process described in the bullet points in Section III(A) one can directly write down the equations to derive  $P(t_m, M | \theta, \ell)$ . The ordering is ignored at first, and false positives are modelled with the binary variable  $f_P = 0/1$ , to indicate that it is activated or not. When a click is spurious  $f_P = 1$ , and when intentional  $f_P = 0$ . Likewise the false negatives are represented with the binary variable  $f_N = 0/1$ . If an intentional click is ignored  $f_N = 1$ , otherwise  $f_N = 0$ . For one click time that was received:

$$\begin{aligned}
 P(t_m | \theta, \ell) &= P(t_m, f_P = 1 | \theta, \ell) + P(t_m, f_P = 0 | \theta, \ell) \\
 &= P(t_m | \theta, f_P = 1, \ell) \cdot P(f_P = 1 | \theta, \ell) \\
 &\quad + P(t_m | \theta, f_P = 0, \ell) \cdot P(f_P = 0 | \theta, \ell) \\
 &= \frac{1}{T} \cdot g + \mathcal{N}(t_m | \theta, \ell) \cdot (1 - g) \\
 &= \frac{1}{T} \cdot g + \mathcal{N}(t_m, f_N = 0 | \theta, \ell) \cdot (1 - g) \\
 &= \frac{1}{T} \cdot g + \mathcal{N}(t_m | f_N = 0, \theta, \ell) \cdot (1 - g) \cdot P(f_N = 0 | \theta, \ell) \\
 &= \frac{1}{T} \cdot g + \mathcal{N}(t_m | f_N = 0, \theta, \ell) \cdot (1 - g) \cdot (1 - f)
 \end{aligned}$$

The integral over  $t_m$  is then:

$$\int_{-\infty}^{\infty} P(t_m | \theta, \ell) dt_m = 1 - f \cdot (1 - g). \quad (2)$$

The outstanding hypothesis is the one where nothing is received. This hypothesis has a probability of  $f \cdot (1 - g)$ . That is  $P(t_m = \emptyset | \theta, \ell) = f \cdot (1 - g)$ .

All the click times are assumed independent, so that:

$$P(\mathbf{t}, M | \theta, \ell) \propto \prod_{m=1}^M P(t_m | \theta, \ell). \quad (3)$$

The constant  $M!$  is then included to accommodate the constraint  $t_1 < t_2 \dots < t_M$  to normalise the integral  $\int_{-\infty}^{\infty} P(\mathbf{t}, M | \theta, \ell) d\mathbf{t} = 1/M!$ .

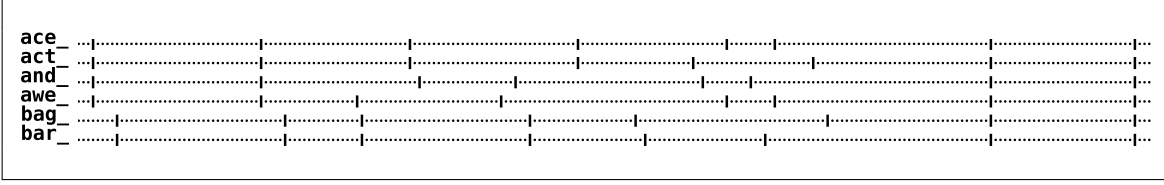

Fig. 2. A visualisation of the binary codes associated with some words.

### III. RECURSION ALGORITHM FOR EFFICIENT CLICK-TIMING INFERENCE

The recursion algorithm for Equation ?? is provided in Table I.

### IV. TRAINING THE CLICK-TIMING MODEL

Online adaptation of this model is done based on the last  $w_{\text{offset}}$  word selections corresponding to the letter sequence  $\{\ell_1^*, \dots, \ell_H^*\}$ . This letter sequence corresponds to a sequence of received click-time ensembles  $\{\{t_1^*, M_1^*\}, \dots, \{t_H^*, M_H^*\}\}$ . An online-learning rate is included to limit the influence of erroneous word selections.

The E-M algorithm is specifically used to compute the maximum-a-posteriori (MAP) estimates  $\theta^*$  of our parameters  $\theta$ . Only true positive click times should contribute to the kernel-density estimation, which results in the following mixture model:

$$P(t_m | \mathbf{z}, \ell, \mathbf{t}^*, \sigma_K) = \frac{\sum_{h, \mathbf{z}^*} \frac{\pi_{h\mathbf{z}^*}}{\sigma_K} \mathcal{N}\left(\frac{t_{m\ell\mathbf{z}} - t_{h\mathbf{z}^*}^*}{\sigma_K} | 0, 1\right)}{\sum_{h, \mathbf{z}^*} \pi_{h\mathbf{z}^*}}, \quad (4)$$

where  $t_{h\mathbf{z}^*}^*$  corresponds to the normalised click-time associated with  $\ell_h^*$  (already selected). Each true positive is weighted by  $\pi_{h\mathbf{z}^*}$ , where, by definition,  $\pi_{h\mathbf{z}^*} \in (0, 1)$ . Each hypothesis contained in  $\mathbf{z}^*$  stipulates which repetition  $r^*$  of  $\ell_h^*$  is responsible for a positive. This enables click-time normalisation, which involves subtracting the corresponding starting time of the sound file from the stored letter time. Likewise, the newly received click-time  $t_m$  is normalised by subtracting the starting time of audio file corresponding to  $\ell$  and  $r$  that is specified by  $\mathbf{z}$ .

It is computationally expensive to train  $\sigma_K$ . A well known approximation amounts to firstly approximating the non-parametric distribution with a Gaussian distribution (by using the E-M algorithm in our case). Secondly, the standard deviation of the latter Gaussian is scaled according to the *normal-scale rule*, in order to compute  $\sigma_K$  [?].

When updating Equation 18, Equation 4 will be used instead of the Gaussian we have used before. The training procedure is followed every-time a new word is selected. Table II summarises the E-M update equations for our application, where the same generic notation defined in [?] were used to do the derivations. At convergence, the Gaussian click-time parameters  $\{\Delta, \sigma\}$  and the switch noise parameters  $\{f, \lambda\}$  are set. These point estimates  $\theta^*$  of the parameters are regularised by the fixed hyper-parameters  $\alpha$  (see Figure ??).

The hyper-parameters were chosen to allow for a broad range of parameters to be learned. Their effect also naturally wears off as more training samples accumulate. We specifically used  $a_\lambda = 1.5$ ,  $b_\lambda = 60$ ,  $a_f = 2$ ,  $b_f = 10$ ,  $\Delta_0 = 0.1$  s,  $\kappa = 0.01$ ,  $a_\beta = 2$ , and  $b_\beta = 0.001$  during the application of the E-M algorithm in our simulations and final user trials.

After applying the E-M algorithm, each of the parameters listed in the M step are updated according to the rule  $\theta = (1 - \lambda_{\text{learn}})\theta_{\text{old}} + \lambda_{\text{learn}}\theta_{\text{new}}$ . After this step, the normal-scale rule is applied to compute  $\sigma_K$ .  $\gamma_{\mathbf{z}h}$  from the E step is then recalculated to compute  $\pi_{h\mathbf{z}^*}$  (see the bottom of Table II). To prevent the system becoming too slow, we only use the last 1000 selected letters during training and evaluation.

In Nomon, there are fewer latent variables, allowing for a straightforward application of the normal-scale rule. Online learning is applied by using linear dampening to reduce the effect of previous samples when updating the kernel-density estimator. This effectively uses an exponential distribution to model the importance of previous samples: As time progresses the importance of older samples will decay exponentially, allowing them to be pruned in a natural way. In our case, older samples are considered just as important as the newest of samples during evaluation, implying a Uniform distribution. Future work will involve testing the effect of dampening of older samples in the same way as Nomon.

Some shortcomings inherent to MAP estimation need to be considered. Since MAP estimates are variable under a change of basis, one may achieve better results in some cases by applying a non-linear transform to the basis of the probability distribution that models the parameter at hand [?]. This option has not been explored for this application.

Like all MAP estimates, successful training strongly depends on good initialisation, which is done as follows. First,  $\lambda$  and  $f$  are initialised by measuring the switch noise. The user is then requested to write the word “yes\_” during a calibration phase before starting to use the system for the first time. The E-M procedure is then used to train  $\{\Delta, \sigma\}$  while keeping  $\{f, \lambda\}$  fixed (to the measured values), and setting  $\lambda_{\text{learn}} = 1.0$ . After calibration  $\lambda_{\text{learn}} = 0.3$  and  $\{f, \lambda\}$  are updated according to the words that are selected. Note that most switch manufacturers specify the typical false positive- and negative rate in their documentation, so that they don’t have to be measured. A fairly large degree of flexibility in the measurement accuracy is also automatically allowed through the hyper-parameters.

**Initialise:**

- For each  $\ell$ , construct a matrix  $G_\ell$  of size  $M \times R$ , where  $g_\ell(m, r) = \mathcal{N}(t_m | \theta_{\ell_r})$ .
- Construct a matrix  $\alpha_C$  of size  $(M+1) \times (R+1)$ , where  $\alpha_C(m, r) = 1, \forall (m, r)$ .

**For**  $C = \{1, \dots, \min(R, M)\}$ :

**For**  $r = \{R', \dots, 1\}$ :

**For**  $m = \{M', \dots, 1\}$ :

$\alpha_C(m, r) = g_\ell(m, r) \cdot \alpha_{C-1}(m+1, r+1) + \alpha_C(m, r+1) + \alpha_C(m+1, r)$

$p_{C\ell} = \alpha_C(1, 1)$

where

- $M' = M - C + 1$  and  $R' = R - C + 1$ .
- At the boundaries,  $\alpha_C(M' + 1, r) = 0$  and  $\alpha_C(m, R' + 1) = 0$ .

TABLE I  
THE RECURSION ALGORITHM FOR EQUATION ?? . NOTE THAT THE SIZE OF  $\alpha_C$  DECREASES TO  $M' \times R'$  AS  $C$  INCREASES.

In an ideal Bayesian world, one would integrate out all the parameters (the trainable ones in  $\theta$ ), instead of inferring point estimates of them. However, one should consider the effect of this approximation for each application, which is more severe if there is a lack of training data. We have only a few parameters, and the distributions over them are quite simple, which implies that, in our case, we have ample training data: On average, each word selection leads to about ten click-times that can be used during training. The error bars (standard deviations of the parameter estimates) in many cases decrease with the familiar scale factor  $1/\sqrt{C_{\text{total}}}$  [?], where  $C_{\text{total}}$  is the total number of click-times during training. Thus, 10 initial click times, which quickly accumulates to at least 100, in addition to the relatively slow learning rate of  $\lambda_{\text{learn}} = 0.3$ , and our calibration step are considered adequate steps to ensure ample training data.

In practice it was found that our training procedure tends to cause over smoothing, which limits entry rate. This is a well-known drawback of the kernel-density estimation described above, and becomes more prevalent when the distribution is multimodal, since  $\sigma$  can become quite large, causing  $\sigma_K$  to become large.

In Nomon, it is easier to learn how to click precisely since the procedure (click when the rotating hand reaches noon) is the same for each letter. Firstly, the user has to get used to the rhythm within a channel. The rhythm created within the channel is imprecise compared to Nomon. The time a sound becomes clearly audible might differ from the ideal click-time (determined by the rhythm) with several tens of milliseconds. It is also more difficult to time the letters at the beginning of the audio sequence, even with the added “tick” sound since the user has to tune in on a specific voice. By construction, it can therefore be expected that the click-time distributions in Nomon will be more unimodal than in Ticker, making over-smoothing less of a problem. It is, however, better to have some probability mass associated with all modes in the click-time distribution, than to have only a unimodal distribution.

A future improvement in Ticker may involve choosing a different click-time distribution. A Dirichlet Process could be a possible choice, allowing for a Gaussian Mixture model, where the number of mixture components can be determined automatically in an elegant way.

## V. LANGUAGE MODELLING

Let there be  $D$  words in the dictionary, and let the  $d$ th word  $\mathbf{w}_d$  consist of a sequence of  $S$  letters:  $\mathbf{w}_d = \{\ell_{d1}, \dots, \ell_{dS}\}$ . When necessary, the notation  $\ell_{dsr}$  is used to refer to the  $r$ th repetition of letter  $\ell_{ds}$ . The set of word priors is represented by  $\Pi_0 = \{\pi_1, \dots, \pi_D\}$ , where  $\pi_d$  is the normalised frequency of the  $d$ th word in the dictionary.

A counting variable  $k$  keeps track of the letter index. If at least one click is received at the end of the audio sequence, the system will move on to the next letter, and  $k$  will be incremented. For example, if the user wants to write the word “is\_”,  $k = 1$ , and the user will start by selecting “i” twice during the presentation of the audio sequence. If the system received clicks at the end of the audio sequence,  $k = 2$ , and the posterior probabilities of all words in the dictionary are updated. These probabilities then become the word priors while  $k = 2$ . This update procedure is formalised through Bayes’ rule, which provides new posterior word probabilities each time  $k$  is updated:

$$\begin{aligned} \pi_{k,d} &= P(\mathbf{w}_d | k, \{\mathbf{t}_1, M_1\}, \dots, \{\mathbf{t}_k, M_k\}, \alpha) \\ &= \int_{\theta} P(\mathbf{w}_d | \theta, \mathcal{D}, \alpha) P(\theta | \mathcal{D}, \alpha) d\theta \end{aligned} \quad (17)$$

where  $\mathcal{D}$  denotes the data  $\{k, \{\mathbf{t}_1, M_1\}, \dots, \{\mathbf{t}_k, M_k\}\}$ . Equation 17 can be approximated as follows:

$$\begin{aligned} \pi_{k,d} &\approx P(\mathbf{w}_d | \theta^*, \mathcal{D}, \alpha) P(\theta^* | \mathcal{D}, \alpha) \\ &= \frac{P(\mathbf{t}_k, M_k | \theta^*, \ell_{ds}) \pi_{k-1,d}}{\sum_{d'=1}^D P(\mathbf{t}_k, M_k | \theta^*, \ell_{d's'}) \pi_{k-1,d'}}, \end{aligned} \quad (18)$$

where  $\theta^*$  is a point estimate of the parameters, and  $P(\mathbf{t}_k, M_k | \theta, \ell_{ds})$  can be computed using Equation ??, where the letter indices are:

$$\begin{aligned} s &= k - \left\lfloor \frac{k-1}{|\mathbf{w}_d|} \right\rfloor \cdot |\mathbf{w}_d| \\ s' &= k - \left\lfloor \frac{k-1}{|\mathbf{w}_{d'}|} \right\rfloor \cdot |\mathbf{w}_{d'}|. \end{aligned} \quad (19)$$

The letter index  $s$  depends on  $k$  and  $d$ , and allows  $\pi_{k,d}$  to be updated even if  $k > |\mathbf{w}_d|$ .

For example, if the system has to compute the denominator in Equation 18 for the word “is\_” and  $k = 4$ , then  $s = 1$ , so that  $\ell_{d1} = \text{i}$ .  $P(\mathbf{t}_4, M_4 | \theta, \ell = \text{i})$  will then be

|                                                                                                                                                                                                                                                                  |      |
|------------------------------------------------------------------------------------------------------------------------------------------------------------------------------------------------------------------------------------------------------------------|------|
| <b>Expectation:</b>                                                                                                                                                                                                                                              |      |
| $\gamma_{\hat{\mathbf{z}}h} = P(\hat{\mathbf{z}}   \mathbf{t}_h, \ell_h, \boldsymbol{\theta}^{\text{old}}, \boldsymbol{\alpha}),$                                                                                                                                | (5)  |
| where $\hat{\mathbf{z}} = \{c_r = 1, n_m = 0, M, N, C\}$ . Equation 5 can be derived from Equation ?? for all the observed letters $\{\ell_1, \dots, \ell_H\}$ , with $\pi_{\ell_h} = 1$ . The expected number of true clicks is given by:                       |      |
| $c^* = \sum_{h=1}^H \sum_{\hat{\mathbf{z}}} \gamma_{\hat{\mathbf{z}}h},$                                                                                                                                                                                         | (6)  |
| where $c^* \in [0, RH]$ .                                                                                                                                                                                                                                        |      |
| <b>Maximisation:</b>                                                                                                                                                                                                                                             |      |
| $\boldsymbol{\theta}^{\text{new}} = \arg \max_{\boldsymbol{\theta}} \mathcal{Q}(\boldsymbol{\theta}, \boldsymbol{\theta}^{\text{old}}),$ where                                                                                                                   |      |
| $\mathcal{Q}(\boldsymbol{\theta}, \boldsymbol{\theta}^{\text{old}}) = \ln \pi_{\boldsymbol{\theta}} + \sum_{h=1}^H \sum_{\hat{\mathbf{z}}} \gamma_{\hat{\mathbf{z}}h} \ln P(\mathbf{t}_h, \hat{\mathbf{z}}   \boldsymbol{\theta}, \ell_h, \boldsymbol{\alpha}),$ |      |
| and $P(\mathbf{t}_h, \hat{\mathbf{z}}   \boldsymbol{\theta}, \ell_h, \boldsymbol{\alpha})$ can be derived from Equation ??. Following the maximisation of $\mathcal{Q}(\boldsymbol{\theta}, \boldsymbol{\theta}^{\text{old}})$ ,                                 |      |
| $\Delta = \frac{\kappa \Delta_0 + \Delta^*}{\kappa + c^*},$                                                                                                                                                                                                      | (7)  |
| $\sigma^2 = \frac{2b_{\beta} + \Delta^{**} + \kappa \Delta_0^2 - \Delta^2(\kappa + c^*)}{2a_{\beta} - 1 + c^*}$                                                                                                                                                  | (8)  |
| $\lambda = \frac{a_{\lambda} - 1 + M^* - c^*}{b_{\lambda} + TH},$                                                                                                                                                                                                | (9)  |
| $f = \frac{RH + a_f - 1 - c^*}{RH + a_f + b_f - 2},$                                                                                                                                                                                                             | (10) |
| where                                                                                                                                                                                                                                                            |      |
| $\Delta^* = \sum_{h=1}^H \sum_{\hat{\mathbf{z}}} \gamma_{\hat{\mathbf{z}}h} \cdot \Delta_{\hat{\mathbf{z}}h}^*,$                                                                                                                                                 | (11) |
| $\Delta^{**} = \sum_{h=1}^H \sum_{\hat{\mathbf{z}}} \gamma_{\hat{\mathbf{z}}h} \cdot (\Delta_{\hat{\mathbf{z}}h}^*)^2,$                                                                                                                                          | (12) |
| $M^* = \sum_{h=1}^H M_h,$                                                                                                                                                                                                                                        | (13) |
| $\Delta_{\hat{\mathbf{z}}h}^* = t_{\hat{\mathbf{z}}h} - \mu_{\hat{\mathbf{z}}h},$                                                                                                                                                                                | (14) |
| where $M_h$ is the number of clicks observed during the selection of letter $\ell_h$ , $t_{\hat{\mathbf{z}}h}$ is the observed click time, and $\mu_{\hat{\mathbf{z}}h}$ is beginning of the audio file implied by the labelling $\hat{\mathbf{z}}$ .            |      |
| <b>Kernel bandwidth parameter:</b>                                                                                                                                                                                                                               |      |
| $\pi_{h\mathbf{z}^*} = \frac{\gamma_{\hat{\mathbf{z}}h}}{c^*}$                                                                                                                                                                                                   | (15) |
| $\sigma_K \approx \frac{1.06\sigma}{(c^*)^{0.2}}$                                                                                                                                                                                                                | (16) |

TABLE II

THE E- AND M-STEPS OF THE E-M ALGORITHM, USED TO TRAIN THE PARAMETERS OF TICKER'S NOISE DISTRIBUTIONS. FOLLOWING THE CONVERGENCE OF  $\mathcal{Q}(\boldsymbol{\theta}, \boldsymbol{\theta}^{\text{old}})$ , EQUATIONS 15-16 ARE APPLIED ONCE AS THE LAST STEP OF TRAINING.

computed from Equation ??, and used in Equation 18. The point estimate  $\boldsymbol{\theta}^*$  is updated after a word has been selected - more detail about this approximation method is given in Section IV.

If  $\max(\Pi_k)$  is bigger than a predefined threshold for updating Equation 18,  $\mathbf{w}_d^*$  is selected, where  $\mathbf{w}_d^* = \arg \max(\Pi_k)$ . The selection threshold was chosen to be 0.9 during all the user trials and simulations. That is, if the system is at least 90% certain of the intentional word, it will be selected. Note that using the maximum posterior value in this way is just a heuristic, and there may well be better alternatives. Other heuristics such as the sum of the posterior probabilities of the top few words may be used, for example.

There is an interesting subtlety to be considered: if one has selected three letters, and move on to the next letter in Nomon, all words consisting of less than four characters will be removed from the "word hypothesis space". In our case, all words are considered at all times. We are currently investigating, as we expect that the best approach to use depends on the click-timing distribution. For example, if the user has an excessive average delay  $\Delta$ , one would definitely expect the Ticker approach to result in a higher text-entry rate, because we can depher the delay to the end of a word (similar in argument to when the fast-scan method is better than the slow-scan method in []).

## VI. THE INTERFACE USED FOR THE STEREOPHONIC USER TRIAL

In Figure 2(a),  $E = 5$ , and the corresponding values of  $\phi_e$  are shown under "Stereo locations". Each colour under "Names", "Select letter", and "Tuning in with visual assistance" corresponds to a sound-source location and person. For example, "Cheerful Charlie" (red) always vocalises letters  $a-e$  in the left ear of the user ( $\phi_e = -1$ ). Cheerful Charlie's audio sequence is *abcdedeabc* (also shown in red).

## VII. A NOTE ON BRAIN-COMPUTER INTERFACES (BCI)

In addition, Ticker's resilience to noise makes it an ideal candidate for Brain-Computer Interfaces (BCIs) that translate brain activity into computer actions (e.g. [?], [?], [?]). Due to the noise, text entry rates in BCIs are extremely low [?], [?], [?], [?]. The main contributing factors to such resilience are its predictive texting traits, the customisable language model and its robustness to long click-time delays and false positives. Users can initially make use of the 1-channel configuration, and gradually progress to more channels if applicable. One might have to repeat the alphabet more than once, as mentioned in Section I.

Brain-Computer Interfaces (BCIs) translate brain activity into computer actions (e.g. [?], [?], [?]). To convert brain activity into a signal that can be reliably used to control a switch for a scanning system is difficult as the signal-to-noise ratio is generally low. Several methods have been developed to capture brain activity each with its pros and cons; see [?] for a summary. Two well-known techniques to

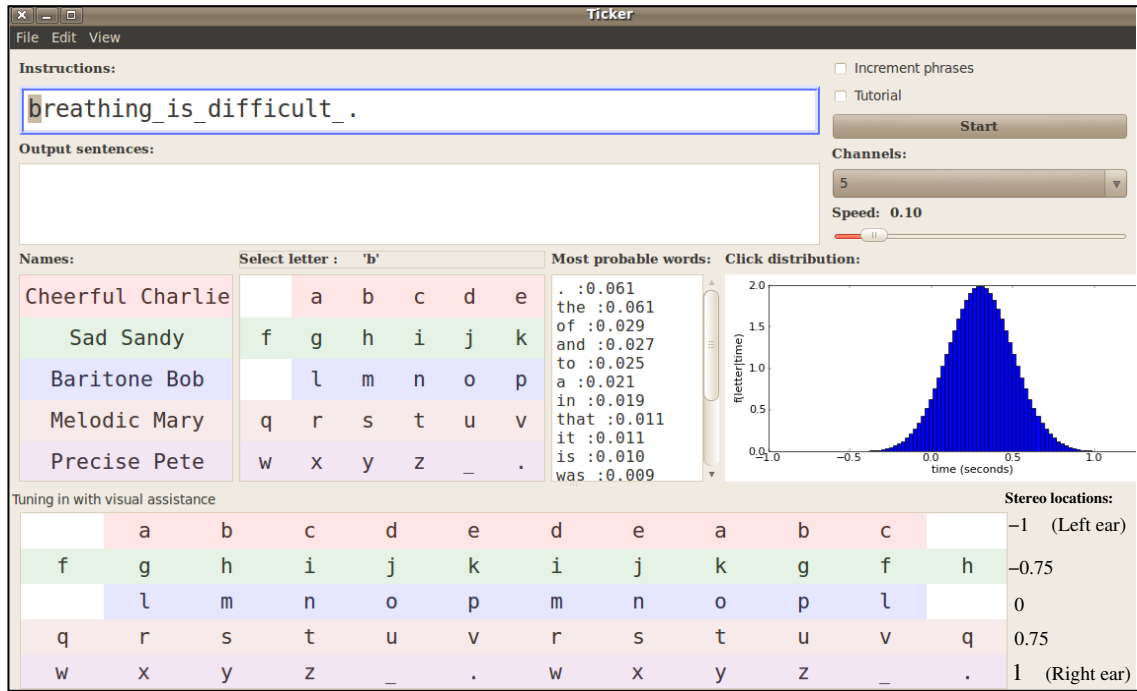

Fig. 3. A visualisation of Ticker in 5-channel mode. Although it is primarily an audio interface, sighted users and instructors can benefit from the visualisation. The audio sequence is shown from top to bottom under “Tuning in”: “fqwaglrxbhm...”.

capture brain-activities are Electroencephalography (EEG) and Functional Magnetic Resonance Imaging (fMRI).

EEG is the predominant technology, where electrodes are placed on the head to measure weak electrical potentials [?]. The technique has low spatial resolution (2-3 cm at best) and requires careful setup. is low (tens of milliseconds). On the other hand, fMRI has high spatial resolution (< 1cm), but high latency (5-8 seconds). EEG can therefore capture a (non-specific) brain signal quickly, whereas fMRI can capture the user’s thoughts with much higher accuracy albeit at a slower rate. Tan and Nijholt [?] mention that 2cm on the cerebral cortex could make it difficult to distinguish if the user is listening to music or conducting a hand motion. Text-entry methods controlled by EEG should therefore be highly resilient to false positives, whereas if controlled by fMRI, they should be highly resilient to long delays.

Due to the noise, text-entry rates are extremely low and typically measured in characters per minute [?]. Blankertz [?] reports a text-entry rate of 7.6 char/min controlling Hex-o-Spell with two switches (only two subjects were tested). Millan et al. [?] mention Hex-o-spell in the context of state-of-the art BCI-spelling devices (in 2010), and as an improvement on the Thought-Translation-Device (with a reported text-entry rate of 0.5 char/min).

In a recent study (2014), Welton et al. [?] reports on the use of Dasher in a BCI context. The pioneering study by Wills and MacKay [?] thought it a viable text-entry method in this context due to its personalised language model and the ability to navigate towards a symbol instead of selecting one symbol at a time (making it more resilient to the noisy EEG data). However, there was uncertainty regarding the

cognitive load of this visually intensive task. Welton et al. [?] tested seven users with a wide range of disabilities. They found that Dasher-BCI was not the answer for all the users, but it may be viable in some cases, and justifies more extensive testing. For example, one user with cerebral palsy who was unable to use the QWERTY keyboard or Dasher-Mouse, could use Dasher-BCI, typing at 4.7 char/min.

Ticker’s resilience to noise makes it an ideal candidate to test for BCI data. The main contributing factors to such resilience are its predictive texting traits, the customisable language model and its robustness to long click-time delays and false positives. Users can initially make use of the one-channel configuration, and gradually progress to more channels if applicable. One might have to repeat the alphabet more than twice for wide click-timing distributions.

#### VIII. A NOTE ON ERROR CORRECTIONS IN TICKER

Error corrections in Ticker are used only in extreme circumstances, as noise compensation allows for a large variety of implicit error correction.

In some cases, two words can strongly compete against each other, especially if the user clicked inaccurately and the intentional word is short. A typical example will be “in\_” and “is\_”. In the 5-channel mode “n” and “s” are nearest neighbours (see Figure 1(a)). If the user clicked slightly inaccurately while aiming for one of these two letters, the probability would typically be split close to equal between the two words to say 0.45 and 0.5. The word would then typically have to be repeated until the confusing letter is reached again, at which point the user would typically resolve his/her previous error.

This aforementioned problem can, of course, be improved by not allowing the letters “n” and “s” to be

neighbours in the first place (see Section ??). A second way to work around this problem would be to change the word-selection heuristic to evaluate the sum of the top three posterior word probabilities instead. The user can then perhaps select between the top three words in some way. This would be slightly complicated, since care has to be taken not to break the user's thought process, in case he/she has to resume with letter selections if the intentional word is not in the top three. It should be noted, however, that during all user trials and simulations it was found to be extremely rare for the intended word not to end up in the top three words, especially by the time the system fails (which is a rare event in itself).

## IX. VIDEOS
